# Supplementary material for: CauseRec: Counterfactual User Sequence Synthesis for Sequential Recommendation
Source: arXiv:2109.05261 source file (2021-09-11)
Supplement: Supplementary file 1 [file 6.Appendix.tex]

\section{Appendix}
\label{sec:appendix}
